# Supplementary material for: Understanding the language of molecules: Predicting pure component parameters for the PC-SAFT equation of state from SMILES
Source: arXiv:2309.12404 ancillary file (2023-09-21)
Supplement: Supplementary file 1 [file SI_SPT_PCSAFT.pdf]

Understanding the language of molecules:  
Predicting pure component parameters for the  
PC-SAFT equation of state from SMILES

Benedikt Winter  
ETH Zurich, EPSE  
Email: [bewinter@ethz.ch](mailto:bewinter@ethz.ch)

Philipp Rehner  
ETH Zurich, EPSE  
Email: [prehner@ethz.ch](mailto:prehner@ethz.ch)

Timm Esper  
University Stuttgart, ITT  
Email: [esper@itt.uni-stuttgart.de](mailto:esper@itt.uni-stuttgart.de)

Johannes Schilling  
ETH Zurich, EPSE  
Email: [jschilling@ethz.ch](mailto:jschilling@ethz.ch)

André Bardow\*  
ETH Zurich, EPSE  
Email: [abardow@ethz.ch](mailto:abardow@ethz.ch)

---

\*Corresponding author. Email: [abardow@ethz.ch](mailto:abardow@ethz.ch)

# 1 Vocab and token training

Table 1: List of tokens and their frequencies.

| Token      | Frequency | Token      | Frequency | Token      | Frequency |
|------------|-----------|------------|-----------|------------|-----------|
| <b>pad</b> | -         | <b>sos</b> | -         | <b>mos</b> | -         |
| <b>eos</b> | -         | <b>c</b>   | 4169      | <b>C</b>   | 13262     |
| <b>(</b>   | 11020     | <b>)</b>   | 11020     | <b>1</b>   | 6145      |
| <b>O</b>   | 8256      | <b>2</b>   | 1545      | <b>=</b>   | 6534      |
| <b>N</b>   | 2384      | <b>n</b>   | 650       | <b>3</b>   | 240       |
| <b>[</b>   | 1824      | <b>]</b>   | 1824      | <b>@</b>   | 345       |
| <b>H</b>   | 609       | <b>F</b>   | 1440      | <b>-</b>   | 738       |
| <b>4</b>   | 49        | <b>S</b>   | 1413      | <b>l</b>   | 1798      |
| <b>/</b>   | 528       | <b>s</b>   | 115       | <b>o</b>   | 93        |
| <b>+</b>   | 588       | <b>5</b>   | 14        | <b>#</b>   | 750       |
| <b>.</b>   | 258       | <b>B</b>   | 714       | <b>r</b>   | 601       |
| <b>\</b>   | 248       | <b>P</b>   | 261       | <b>6</b>   | 2         |
| <b>I</b>   | 191       | <b>a</b>   | 1         | <b>i</b>   | 716       |
| <b>7</b>   | 0         | <b>e</b>   | 8         | <b>K</b>   | 0         |
| <b>8</b>   | 0         | <b>L</b>   | 1         | <b>A</b>   | 1         |
| <b>Z</b>   | 3         | <b>g</b>   | 0         | <b>M</b>   | 0         |
| <b>T</b>   | 11        | <b>t</b>   | 0         | <b>9</b>   | 0         |
| <b>p</b>   | 0         | <b>%</b>   | 0         | <b>0</b>   | 0         |
| <b>V</b>   | 0         | <b>b</b>   | 12        | <b>u</b>   | 11        |
| <b>R</b>   | 5         | <b>X</b>   | 0         | <b>H2O</b> | 0         |
| <b>d</b>   | 3         | <b>G</b>   | 1         | <b>Y</b>   | 2         |
| <b>D</b>   | 0         | <b>y</b>   | 0         | <b>W</b>   | 0         |
| <b>E</b>   | 2         | <b>f</b>   | 3         | <b>h</b>   | 0         |
| <b>m</b>   | 0         | <b>U</b>   | 0         |            |           |

## 2 Derivations of the implicit derivatives of liquid densities and vapor pressures

The equation for the calculation of a liquid density  $\rho_L$  for given temperature  $T$  and pressure  $p$  and model parameters  $\phi$  from an equation of state is

$$f(\rho_L) = p(T, \rho_L, \phi) - p = 0 \quad (1)$$

It is then straightforward to use a Newton step to calculate the derivatives for an already converged value of the liquid density  $\rho_L^*$

$$\rho_L(T, p, \phi) = \rho_L^* - \frac{p(T, \rho_L^*, \phi) - p}{p_\rho(T, \rho_L^*, \phi)} \quad (2)$$

For the calculation of the vapor pressure  $p^{\text{sat}}$  for given temperature  $T$  and model parameters  $\phi$  the equilibrium condition

$$f(p^{\text{sat}}) = \mu_V(T, p^{\text{sat}}, \phi) - \mu_L(T, p^{\text{sat}}, \phi) = 0 \quad (3)$$

needs to be solved. Here,  $\mu_V$  and  $\mu_L$  are the chemical potentials of the liquid and the vapor phase. Applying the newton step from a known vapor pressure  $p^{\text{sat},*}$  yields

$$p^{\text{sat}}(T, \phi) = p^{\text{sat},*} - \frac{\mu_V(T, p^{\text{sat},*}, \phi) - \mu_L(T, p^{\text{sat},*}, \phi)}{v_V(T, p^{\text{sat},*}, \phi) - v_L(T, p^{\text{sat},*}, \phi)} \quad (4)$$

where the thermodynamic identity  $v = \left(\frac{\partial \mu}{\partial p}\right)_T$  was used. The expression can be further simplified by using the molar Helmholtz energy  $a = -pv + \mu$ , as

$$p^{\text{sat}}(T, \phi) = -\frac{a_V(T, p^{\text{sat},*}, \phi) - a_L(T, p^{\text{sat},*}, \phi)}{v_V(T, p^{\text{sat},*}, \phi) - v_L(T, p^{\text{sat},*}, \phi)} \quad (5)$$

If the vapor pressure is calculated from an equation of state, the molar Helmholtz energy and volume are expressed in terms of the density, which then gives the expression shown in the main manuscript

$$p^{\text{sat}}(T, \phi) = -\frac{a(T, \rho_V^*, \phi) - a(T, \rho_L^*, \phi)}{\frac{1}{\rho_V^*} - \frac{1}{\rho_L^*}} \quad (6)$$

### 3 Data Cleaning

In the initial dataset processing, data points with a vapor pressure of 1.00(1) bar at 298.15(100) K were excluded. These entries were deemed to have been erroneously entered. Further refinement was made by removing data points incompatible with the PC-SAFT fitting.

For this refinement, eight models were trained on the dataset over 15 epochs utilizing a SmoothL1 loss function. This particular loss function was chosen to mitigate the undue influence of outliers compared to using an MSE loss. Subsequent to this training, any data points that exhibited a training loss greater than 0.5 in the remaining dataset were removed.

As a result of this data cleaning process, 21 456 out of 233 988 data points were removed. This left the remaining dataset with 160 186 vapor pressure data points with to 12 019 molecules and 52 343 liquid density data points corresponding to 2067 molecules. Manual inspection of the discarded data points largely confirmed the removal of data that appeared unreasonable or anomalous. For examples, see Figure S1. In the course of the data cleaning, several types of errors were identified. Primarily were data series that appeared erroneous, either due to their stark deviation from expected values or patterns inconsistent with related data (Figure S1a-S1b). Additionally, we identified instances of data scattering, which could potentially hinder model training (Figure S1c-S1d).

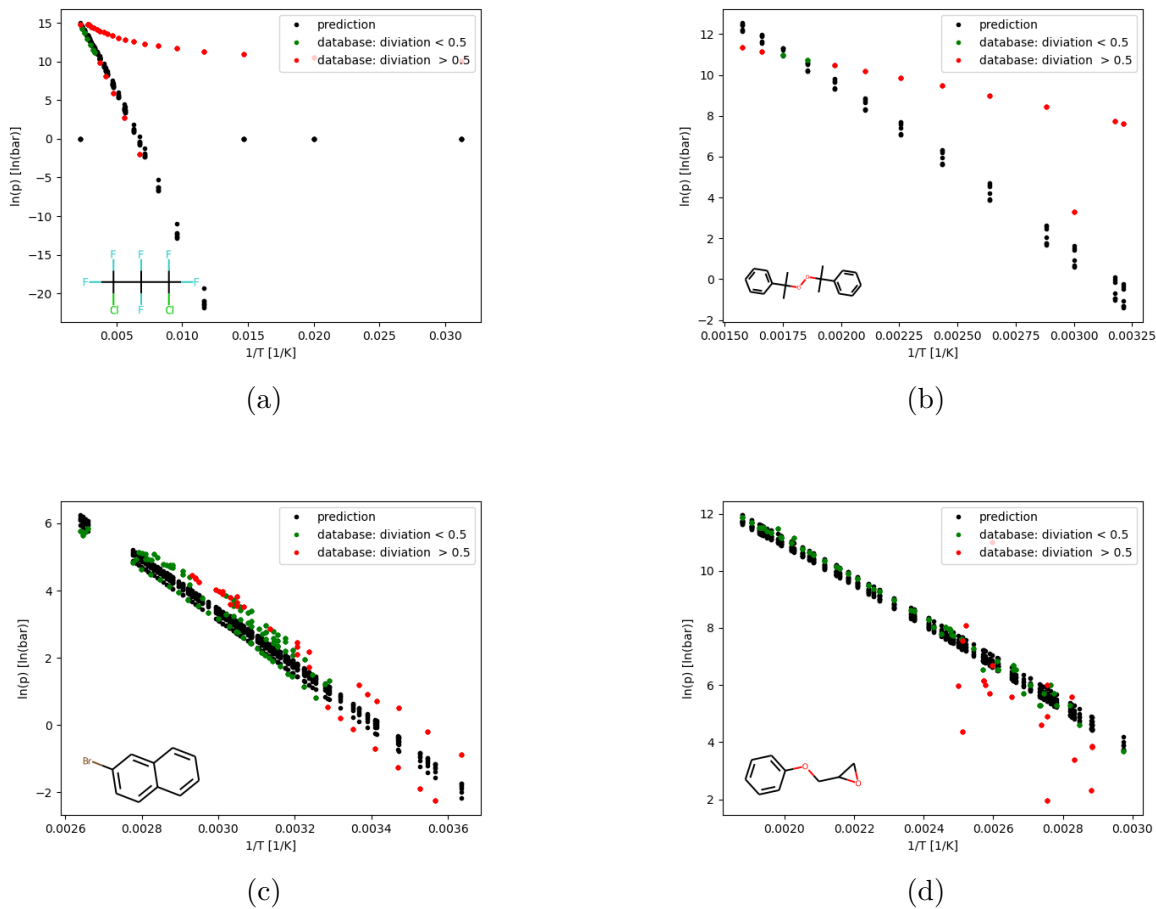

Figure S1: Examples for topical errors in the remaining data identified by our cleaning step. If the prediction for vapor pressure is 0, the predicted state is supercritical.

## 4 Receiver operating characteristic curve

The Receiver Operating Characteristic (ROC) curve is a graphical representation used to evaluate the performance of binary classification models. It plots the true positive rate against the false positive rate at various threshold settings, illustrating the trade-off between sensitivity and specificity. An area under the ROC curve (AUC) value of 1 represents a perfect model, while an AUC value of 0.5 suggests a model no better than random guessing.

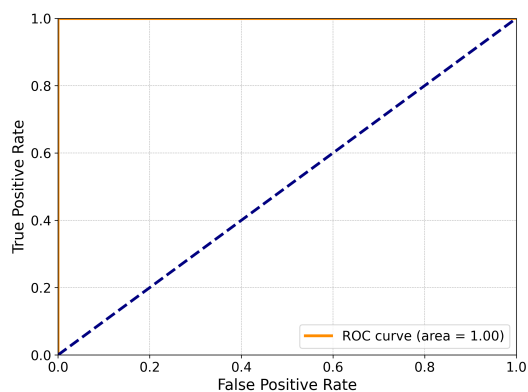

(a) association likelihood

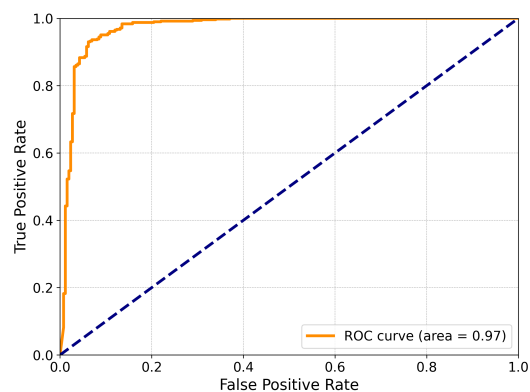

(b) polarity likelihood

Figure S2: ROC curves for the association and polarity likelihood

In our analysis, the ROC curve for the association likelihood exhibits an impeccable performance, with an AUC of 1 (Figure S2a). This suggests that the model can flawlessly differentiate between the positive and negative classes for this likelihood. Given that association is determined by the presence of hydrogen bonding groups, which can be easily discerned from SMILES codes, this outcome is not surprising. Conversely, the ROC curve for the polarity likelihood, though not perfect, demonstrates still an outstanding performance, with an AUC of 0.97 (Figure S2b). Since polarity is determined based on discrete decisions within a continuous space, a perfect representation should not be expected.

## 5 Molecular Families

Table 2: List of names, their SMILES notations, and families of the validation set that could be grouped into families

| Name                            | SMILES                                 | Family   |
|---------------------------------|----------------------------------------|----------|
| lauricacid                      | <chem>CCCCCCCCCCCC(=O)O</chem>         | Acids    |
| pentanoicacid                   | <chem>CCCCC(=O)O</chem>                | Acids    |
| tridecanoicacid                 | <chem>CCCCCCCCCCCCC(=O)O</chem>        | Acids    |
| heptanoicacid                   | <chem>CCCCCCC(=O)O</chem>              | Acids    |
| methacrylicacid                 | <chem>C=C(C)C(=O)O</chem>              | Acids    |
| caprylicacid                    | <chem>CCCCCCCC(=O)O</chem>             | Acids    |
| nonanoicacid                    | <chem>CCCCCCCCC(=O)O</chem>            | Acids    |
| capricacid                      | <chem>CCCCCCCCCC(=O)O</chem>           | Acids    |
| hexanoicacid                    | <chem>CCCCCC(=O)O</chem>               | Acids    |
| 3-methylbutanoicacid            | <chem>CC(C)CC(=O)O</chem>              | Acids    |
| arachidicacid                   | <chem>CCCCCCCCCCCCCCCCCCCC(=O)O</chem> | Acids    |
| 2-ethylhexanoicacid             | <chem>CCCCC(CC)C(=O)O</chem>           | Acids    |
| undecanoicacid                  | <chem>CCCCCCCCCCC(=O)O</chem>          | Acids    |
| myristicacid                    | <chem>CCCCCCCCCCCCC(=O)O</chem>        | Acids    |
| pentadecanoicacid               | <chem>CCCCCCCCCCCCCCC(=O)O</chem>      | Acids    |
| stearicacid                     | <chem>CCCCCCCCCCCCCCCCCCC(=O)O</chem>  | Acids    |
| 2-methylpropanoicacid           | <chem>CC(C)C(=O)O</chem>               | Acids    |
| palmiticacid                    | <chem>CCCCCCCCCCCCCCCC(=O)O</chem>     | Acids    |
| butyricacid                     | <chem>CCCC(=O)O</chem>                 | Acids    |
| pivalicacid                     | <chem>CC(C)(C)C(=O)O</chem>            | Acids    |
| 2-heptanol                      | <chem>CCCCCC(C)O</chem>                | Alcohols |
| 1,3-butanediol                  | <chem>CC(O)CCO</chem>                  | Alcohols |
| 2-methyl-2,4-pentanediol        | <chem>CC(O)CC(C)(C)O</chem>            | Alcohols |
| 2,3-butanediol                  | <chem>CC(O)C(C)O</chem>                | Alcohols |
| 1-butanol                       | <chem>CCCCO</chem>                     | Alcohols |
| tert-butanol                    | <chem>CC(C)(C)O</chem>                 | Alcohols |
| 2-octanol                       | <chem>CCCCCCC(C)O</chem>               | Alcohols |
| 2-methyl-1-propanol             | <chem>CC(C)CO</chem>                   | Alcohols |
| 2,2,4-trimethyl-1,3-pentanediol | <chem>CC(C)C(O)C(C)(C)CO</chem>        | Alcohols |
| 3-methyl-1-butanol              | <chem>CC(C)CCO</chem>                  | Alcohols |
| 1-pentanol                      | <chem>CCCCCO</chem>                    | Alcohols |
| 1-hexanol                       | <chem>CCCCCCO</chem>                   | Alcohols |
| 1-heptanol                      | <chem>CCCCCCCO</chem>                  | Alcohols |
| 1-octanol                       | <chem>CCCCCCCCO</chem>                 | Alcohols |
| 1-nonanol                       | <chem>CCCCCCCCCO</chem>                | Alcohols |
| 1-undecanol                     | <chem>CCCCCCCCCCC</chem>               | Alcohols |
| 1-dodecanol                     | <chem>CCCCCCCCCCCC</chem>              | Alcohols |
| n-tridecanol                    | <chem>CCCCCCCCCCCCC</chem>             | Alcohols |
| 1-tetradecanol                  | <chem>CCCCCCCCCCCCC</chem>             | Alcohols |
| 1-hexadecanol                   | <chem>CCCCCCCCCCCCCCC</chem>           | Alcohols |
| 1-octadecanol                   | <chem>CCCCCCCCCCCCCCCC</chem>          | Alcohols |
| 3-methyl-2-butanol              | <chem>CC(C)C(C)O</chem>                | Alcohols |
| 4-methyl-2-pentanol             | <chem>CC(C)CC(C)O</chem>               | Alcohols |
| 1-decanol                       | <chem>CCCCCCCCCO</chem>                | Alcohols |
| diethyleneglycol                | <chem>OCCOCCO</chem>                   | Alcohols |
| triethyleneglycol               | <chem>OCCOCCOCCO</chem>                | Alcohols |
| 3-methyl-3-pentanol             | <chem>CCC(C)(O)CC</chem>               | Alcohols |
| 2-methyl-1-pentanol             | <chem>CCCC(C)CO</chem>                 | Alcohols |

Table 2: List of names, their SMILES notations, and families of the validation set that could be grouped into families

| Name                              | SMILES                       | Family    |
|-----------------------------------|------------------------------|-----------|
| 2-methyl-1-butanol                | <chem>CCC(C)CO</chem>        | Alcohols  |
| 2-ethyl-1-hexanol                 | <chem>CCCCC(CC)CO</chem>     | Alcohols  |
| 2-pentanol                        | <chem>CCCC(C)O</chem>        | Alcohols  |
| 3-hexanol                         | <chem>CCCC(O)CC</chem>       | Alcohols  |
| cyclohexanol                      | <chem>OC1CCCCC1</chem>       | Alcohols  |
| 1,2-dihydroxybenzene pyrocatechol | <chem>Oc1ccccc1O</chem>      | Alcohols  |
| 1,10-decanediol                   | <chem>OCCCCCCCCCCO</chem>    | Alcohols  |
| 2-butanol                         | <chem>CCC(C)O</chem>         | Alcohols  |
| 1,3-dihydroxybenzene resorcinol   | <chem>Oc1ccc(O)c1</chem>     | Alcohols  |
| 1,6-hexanediol                    | <chem>OCCCCCO</chem>         | Alcohols  |
| 1,2-butanediol                    | <chem>CCC(O)CO</chem>        | Alcohols  |
| 1,4-butanediol                    | <chem>OCCCCO</chem>          | Alcohols  |
| 2-methyl-1-hexanol                | <chem>CCCCC(C)CO</chem>      | Alcohols  |
| 3-pentanol                        | <chem>CCC(O)CC</chem>        | Alcohols  |
| 2-hexanol                         | <chem>CCCCC(C)O</chem>       | Alcohols  |
| tetraethyleneglycol               | <chem>OCCOCCOCCOCCO</chem>   | Alcohols  |
| tert-pentanol                     | <chem>CCC(C)(C)O</chem>      | Alcohols  |
| 3-methylbutyraldehyde             | <chem>CC(C)CC=O</chem>       | Aldehydes |
| 2-methylpropanal                  | <chem>CC(C)C=O</chem>        | Aldehydes |
| n-decanal                         | <chem>CCCCCCCCCCC=O</chem>   | Aldehydes |
| valeraldehyde                     | <chem>CCCCC=O</chem>         | Aldehydes |
| methacrolein                      | <chem>C=C(C)C=O</chem>       | Aldehydes |
| nonanal                           | <chem>CCCCCCCCC=O</chem>     | Aldehydes |
| hexanal                           | <chem>CCCCC=O</chem>         | Aldehydes |
| undecanaldehyde                   | <chem>CCCCCCCCCCC=O</chem>   | Aldehydes |
| octanal                           | <chem>CCCCCCCC=O</chem>      | Aldehydes |
| heptanal                          | <chem>CCCCCCC=O</chem>       | Aldehydes |
| 2-methylbutyraldehyde             | <chem>CCC(C)C=O</chem>       | Aldehydes |
| 2-phenylpropionaldehyde           | <chem>CC(C=O)c1ccccc1</chem> | Aldehydes |
| butyraldehyde                     | <chem>CCCC=O</chem>          | Aldehydes |
| 2,3-dimethylbutane                | <chem>CC(C)C(C)C</chem>      | Alkanes   |
| dodecane                          | <chem>CCCCCCCCCCCC</chem>    | Alkanes   |
| 2-methylpropane                   | <chem>CC(C)C</chem>          | Alkanes   |
| n-butane                          | <chem>CCCC</chem>            | Alkanes   |
| n-undecane                        | <chem>CCCCCCCCCCCC</chem>    | Alkanes   |
| 2,3-dimethylpentane               | <chem>CCC(C)C(C)C</chem>     | Alkanes   |
| 2,2-dimethylpentane               | <chem>CCCC(C)(C)C</chem>     | Alkanes   |
| 2,2,3-trimethylbutane             | <chem>CC(C)C(C)(C)C</chem>   | Alkanes   |
| 2,4-dimethylhexane                | <chem>CCC(C)CC(C)C</chem>    | Alkanes   |
| 3-methylpentane                   | <chem>CCC(C)CC</chem>        | Alkanes   |
| 2,3-dimethylhexane                | <chem>CCCC(C)C(C)C</chem>    | Alkanes   |
| 2-methylpentane                   | <chem>CCCC(C)C</chem>        | Alkanes   |
| hexane                            | <chem>CCCCCC</chem>          | Alkanes   |
| 2-methylheptane                   | <chem>CCCCC(C)C</chem>       | Alkanes   |
| 3-methylheptane                   | <chem>CCCCC(C)CC</chem>      | Alkanes   |
| 2-methylhexane                    | <chem>CCCCC(C)C</chem>       | Alkanes   |
| pentane                           | <chem>CCCCC</chem>           | Alkanes   |
| heptane                           | <chem>CCCCCCC</chem>         | Alkanes   |
| 2-methyloctane                    | <chem>CCCCCCC(C)C</chem>     | Alkanes   |
| octane                            | <chem>CCCCCCCC</chem>        | Alkanes   |
| nonane                            | <chem>CCCCCCCCC</chem>       | Alkanes   |

Table 2: List of names, their SMILES notations, and families of the validation set that could be grouped into families

| Name                            | SMILES                                                 | Family  |
|---------------------------------|--------------------------------------------------------|---------|
| 2-methylbutane                  | <chem>CCC(C)C</chem>                                   | Alkanes |
| 4-methylheptane                 | <chem>CCCC(C)CCC</chem>                                | Alkanes |
| decane                          | <chem>CCCCCCCCC</chem>                                 | Alkanes |
| 3,3-dimethylpentane             | <chem>CCC(C)(C)CC</chem>                               | Alkanes |
| 2,7-dimethyloctane              | <chem>CC(C)CCCC(C)C</chem>                             | Alkanes |
| squalane                        | <chem>CC(C)CCCC(C)CCCC(C)CCCC(C)CCCC(C)CCCC(C)C</chem> | Alkanes |
| 3-methylhexane                  | <chem>CCCC(C)CC</chem>                                 | Alkanes |
| 2,5-dimethylhexane              | <chem>CC(C)CCC(C)C</chem>                              | Alkanes |
| 2,2,5-trimethylhexane           | <chem>CC(C)CCC(C)(C)C</chem>                           | Alkanes |
| 2,4-dimethylpentane             | <chem>CC(C)CC(C)C</chem>                               | Alkanes |
| 2,2,4-trimethylpentane          | <chem>CC(C)CC(C)(C)C</chem>                            | Alkanes |
| 2,2-dimethylbutane              | <chem>CCC(C)(C)C</chem>                                | Alkanes |
| 2,2,4,4,6,8,8-heptamethylnonane | <chem>CC(CC(C)(C)C)CC(C)(C)CC(C)(C)C</chem>            | Alkanes |
| octadecane                      | <chem>CCCCCCCCCCCCCCCCC</chem>                         | Alkanes |
| tetradecane                     | <chem>CCCCCCCCCCCCC</chem>                             | Alkanes |
| tridecane                       | <chem>CCCCCCCCCCCCC</chem>                             | Alkanes |
| octacosane                      | <chem>CCCCCCCCCCCCCCCCCCCCCCCCCCCCCCCC</chem>          | Alkanes |
| heptacosane                     | <chem>CCCCCCCCCCCCCCCCCCCCCCCCCCCCCCCC</chem>          | Alkanes |
| pentacosane                     | <chem>CCCCCCCCCCCCCCCCCCCCCCCCCCCCCCCC</chem>          | Alkanes |
| tetracosane                     | <chem>CCCCCCCCCCCCCCCCCCCCCCCCCCCCCCCC</chem>          | Alkanes |
| eicosane                        | <chem>CCCCCCCCCCCCCCCCCCCCCCCCCCCC</chem>              | Alkanes |
| nonadecane                      | <chem>CCCCCCCCCCCCCCCCCCCCCCCCC</chem>                 | Alkanes |
| 3-ethylpentane                  | <chem>CCC(CC)CC</chem>                                 | Alkanes |
| heptadecane                     | <chem>CCCCCCCCCCCCCCCCC</chem>                         | Alkanes |
| 2,2-dimethylpropane             | <chem>CC(C)(C)C</chem>                                 | Alkanes |
| hexadecane                      | <chem>CCCCCCCCCCCCCCCCC</chem>                         | Alkanes |
| pentadecane                     | <chem>CCCCCCCCCCCCCCCCC</chem>                         | Alkanes |
| 3,3-diethylpentane              | <chem>CCC(CC)(CC)CC</chem>                             | Alkanes |
| 4-methyl-1-pentene              | <chem>C=CCC(C)C</chem>                                 | Alkenes |
| 1-butene                        | <chem>C=CCC</chem>                                     | Alkenes |
| 1,3-butadiene                   | <chem>C=CC=C</chem>                                    | Alkenes |
| 3-methyl-1-hexene               | <chem>C=CC(C)CCC</chem>                                | Alkenes |
| 3-methyl-1-butene               | <chem>C=CC(C)C</chem>                                  | Alkenes |
| 2,3-dimethyl-2-butene           | <chem>CC(C)=C(C)C</chem>                               | Alkenes |
| dimethylallene                  | <chem>C=C=C(C)C</chem>                                 | Alkenes |
| 2,4,4-trimethyl-1-pentene       | <chem>C=C(C)CC(C)(C)C</chem>                           | Alkenes |
| 1,4-pentadiene                  | <chem>C=CCC=C</chem>                                   | Alkenes |
| 2-methyl-1-butene               | <chem>C=C(C)CC</chem>                                  | Alkenes |
| 2,3-dimethyl-1-butene           | <chem>C=C(C)C(C)C</chem>                               | Alkenes |
| 2-methyl-2-butene               | <chem>CC=C(C)C</chem>                                  | Alkenes |
| isobutylene                     | <chem>C=C(C)C</chem>                                   | Alkenes |
| 1,4-cyclohexadiene              | <chem>C1=CCC=CC1</chem>                                | Alkenes |
| 1,3-cyclopentadiene             | <chem>C1=CCC=C1</chem>                                 | Alkenes |
| 2-methyl-2-pentene              | <chem>CCC=C(C)C</chem>                                 | Alkenes |
| 2-methyl-1-pentene              | <chem>C=C(C)CCC</chem>                                 | Alkenes |
| 1-pentene                       | <chem>C=CCCC</chem>                                    | Alkenes |
| isoprene                        | <chem>C=CC(=C)C</chem>                                 | Alkenes |

Table 2: List of names, their SMILES notations, and families of the validation set that could be grouped into families

| Name                                  | SMILES                           | Family  |
|---------------------------------------|----------------------------------|---------|
| 1-hexene                              | <chem>C=CCCCC</chem>             | Alkenes |
| 1,5-hexadiene                         | <chem>C=CCCC=C</chem>            | Alkenes |
| 1-hexadecene                          | <chem>C=CCCCCCCCCCCCCCC</chem>   | Alkenes |
| 2,4,4-trimethyl-2-pentene             | <chem>CC(C)=CC(C)(C)C</chem>     | Alkenes |
| 1-tetradecene                         | <chem>C=CCCCCCCCCCCCC</chem>     | Alkenes |
| 1-dodecene                            | <chem>C=CCCCCCCCCCC</chem>       | Alkenes |
| 1-undecene                            | <chem>C=CCCCCCCCC</chem>         | Alkenes |
| 1-octadecene                          | <chem>C=CCCCCCCCCCCCCCCCC</chem> | Alkenes |
| 1-decene                              | <chem>C=CCCCCCCC</chem>          | Alkenes |
| 1-nonene                              | <chem>C=CCCCCCC</chem>           | Alkenes |
| 1-octene                              | <chem>C=CCCCCC</chem>            | Alkenes |
| 1-heptene                             | <chem>C=CCCCC</chem>             | Alkenes |
| 2-butyne                              | <chem>CC#CC</chem>               | Alkynes |
| 1-butyne                              | <chem>C#CCC</chem>               | Alkynes |
| 1-pentyne                             | <chem>C#CCCC</chem>              | Alkynes |
| 1-hexyne                              | <chem>C#CCCCC</chem>             | Alkynes |
| 3-hexyne                              | <chem>CCC#CCC</chem>             | Alkynes |
| 1-heptyne                             | <chem>C#CCCCC</chem>             | Alkynes |
| 1-octyne                              | <chem>C#CCCCC</chem>             | Alkynes |
| 1-nonyne                              | <chem>C#CCCCCCC</chem>           | Alkynes |
| 1-buten-3-yne                         | <chem>C#CC=C</chem>              | Alkynes |
| 2-hexyne                              | <chem>CC#CCCC</chem>             | Alkynes |
| diethylenetriamine                    | <chem>NCCNCCN</chem>             | Amines  |
| n-(2-aminoethyl)ethanolamine          | <chem>NCCNCCO</chem>             | Amines  |
| pyrrole                               | <chem>c1cc[nH]c1</chem>          | Amines  |
| triethanolamine(tea)                  | <chem>OCCN(CCO)CCO</chem>        | Amines  |
| 2,2'-diethanolamine(dea)              | <chem>OCCNCCO</chem>             | Amines  |
| 1-octanamine                          | <chem>CCCCCCCCN</chem>           | Amines  |
| n-(2-aminoethyl)piperazine            | <chem>NCCN1CCNCC1</chem>         | Amines  |
| indole                                | <chem>c1ccc2[nH]ccc2c1</chem>    | Amines  |
| diglycolamine(dga)                    | <chem>NCCOCCO</chem>             | Amines  |
| 1,6-hexanediamine                     | <chem>NCCCCCN</chem>             | Amines  |
| n-methylcyclohexylamine               | <chem>CNC1CCCCC1</chem>          | Amines  |
| cyclopentylamine                      | <chem>NC1CCCC1</chem>            | Amines  |
| tributylamine                         | <chem>CCCCN(CCCC)CCCC</chem>     | Amines  |
| dibutylamine                          | <chem>CCCCNCCCC</chem>           | Amines  |
| dipropylamine                         | <chem>CCCNCCC</chem>             | Amines  |
| methyldiethylamine                    | <chem>CCN(C)CC</chem>            | Amines  |
| triethylamine                         | <chem>CCN(CC)CC</chem>           | Amines  |
| n,n-diethylethanolamine(dem ea)       | <chem>CCN(CC)CCO</chem>          | Amines  |
| n,n-diethylamine                      | <chem>CCNCC</chem>               | Amines  |
| 3-n,n-dimethylaminopropylamine        | <chem>CN(C)CCCN</chem>           | Amines  |
| n,n,n',n'-tetramethylethylene diamine | <chem>CN(C)CCN(C)C</chem>        | Amines  |
| n,n-dimethylethanolamine(d mmea)      | <chem>CN(C)CCO</chem>            | Amines  |
| butylamine                            | <chem>CCCCN</chem>               | Amines  |
| 1-aminopentane                        | <chem>CCCCCN</chem>              | Amines  |
| hexylamine                            | <chem>CCCCCCN</chem>             | Amines  |
| heptylamine                           | <chem>CCCCCCCN</chem>            | Amines  |

Table 2: List of names, their SMILES notations, and families of the validation set that could be grouped into families

| Name                                 | SMILES                                 | Family                |
|--------------------------------------|----------------------------------------|-----------------------|
| methyldiethanolamine(mdea)           | <chem>CN(CCO)CCO</chem>                | Amines                |
| n-methylpiperidine                   | <chem>CN1CCCCC1</chem>                 | Amines                |
| trioctylamine                        | <chem>CCCCCCCCCN(CCCCCCCC)CCCCC</chem> | Amines                |
|                                      | <chem>CCC</chem>                       |                       |
| cyclohexylamine                      | <chem>NC1CCCCC1</chem>                 | Amines                |
| tripropylamine                       | <chem>CCCN(CCC)CCC</chem>              | Amines                |
| pyrazine                             | <chem>c1cnccn1</chem>                  | Amines                |
| tert-butylamine                      | <chem>CC(C)(C)N</chem>                 | Amines                |
| piperidine                           | <chem>C1CCNCC1</chem>                  | Amines                |
| diisopropanolamine(dipa)             | <chem>CC(O)CNCC(C)O</chem>             | Amines                |
| diisopropylamine                     | <chem>CC(C)NC(C)C</chem>               | Amines                |
| dicyclohexylamine                    | <chem>C1CCC(NC2CCCCC2)CC1</chem>       | Amines                |
| hexamethyleneimine                   | <chem>C1CCCNCC1</chem>                 | Amines                |
| n,n-dimethylacetamide                | <chem>CC(=O)N(C)C</chem>               | Amines                |
| 2-amino-2-methyl-1-propanol<br>(amp) | <chem>CC(C)(N)CO</chem>                | Amines                |
| 2-methylpropylamine                  | <chem>CC(C)CN</chem>                   | Amines                |
| pyrrolidine                          | <chem>C1CCNC1</chem>                   | Amines                |
| sec-butylamine                       | <chem>CCC(C)N</chem>                   | Amines                |
| alpha-methylstyrene                  | <chem>C=C(C)c1ccccc1</chem>            | Aromatic hydrocarbons |
| p-methylaniline                      | <chem>Cc1ccc(N)cc1</chem>              | Aromatic hydrocarbons |
| 3,5-dimethylphenol                   | <chem>Cc1cc(C)cc(O)c1</chem>           | Aromatic hydrocarbons |
| phenylhydrazine                      | <chem>NNc1ccccc1</chem>                | Aromatic hydrocarbons |
| hexylbenzene                         | <chem>CCCCCc1ccccc1</chem>             | Aromatic hydrocarbons |
| aniline                              | <chem>Nc1ccccc1</chem>                 | Aromatic hydrocarbons |
| 2,4-dimethylaniline                  | <chem>Cc1ccc(N)c(C)c1</chem>           | Aromatic hydrocarbons |
| p-chlorotoluene                      | <chem>Cc1ccc(Cl)cc1</chem>             | Aromatic hydrocarbons |
| heptylbenzene                        | <chem>CCCCCCCc1ccccc1</chem>           | Aromatic hydrocarbons |
| p-xylene                             | <chem>Cc1ccc(C)cc1</chem>              | Aromatic hydrocarbons |
| aceticacidbenzylester                | <chem>CC(=O)OCc1ccccc1</chem>          | Aromatic hydrocarbons |
| benzoicacid                          | <chem>O=C(O)c1ccccc1</chem>            | Aromatic hydrocarbons |
| p-methyl-styrene                     | <chem>C=Cc1ccc(C)cc1</chem>            | Aromatic hydrocarbons |
| octylbenzene                         | <chem>CCCCCCCCc1ccccc1</chem>          | Aromatic hydrocarbons |
| 1,3-diethylbenzene                   | <chem>CCc1cccc(CC)c1</chem>            | Aromatic hydrocarbons |
| 3-methylstyrene;3-vinyltolue<br>ne;  | <chem>C=Cc1cccc(C)c1</chem>            | Aromatic hydrocarbons |
| styrene                              | <chem>C=Cc1ccccc1</chem>               | Aromatic hydrocarbons |
| benzylbenzoate                       | <chem>O=C(OCc1ccccc1)c1ccccc1</chem>   | Aromatic hydrocarbons |
| nonylbenzene                         | <chem>CCCCCCCCCc1ccccc1</chem>         | Aromatic hydrocarbons |
| 1,2,4-trimethylbenzene               | <chem>Cc1ccc(C)c(C)c1</chem>           | Aromatic hydrocarbons |
| 1-phenyldecane                       | <chem>CCCCCCCCCc1ccccc1</chem>         | Aromatic hydrocarbons |
| 4-isopropyltoluene                   | <chem>Cc1ccc(C(C)C)cc1</chem>          | Aromatic hydrocarbons |
| 1-phenylundecane                     | <chem>CCCCCCCCCCCCc1ccccc1</chem>      | Aromatic hydrocarbons |
| 2-ethylphenol                        | <chem>CCc1ccccc1O</chem>               | Aromatic hydrocarbons |
| 1-phenyldodecane                     | <chem>CCCCCCCCCCCCCc1ccccc1</chem>     | Aromatic hydrocarbons |
| 1-ethyl-2-methylbenzene              | <chem>CCc1ccccc1C</chem>               | Aromatic hydrocarbons |
| 2,4,6-trimethylpyridine              | <chem>Cc1cc(C)nc(C)c1</chem>           | Aromatic hydrocarbons |
| 1-ethyl-4-methylbenzene              | <chem>CCc1ccc(C)cc1</chem>             | Aromatic hydrocarbons |
| 1-ethyl-3-methylbenzene              | <chem>CCc1cccc(C)c1</chem>             | Aromatic hydrocarbons |
| 1-ethylnaphthalene                   | <chem>CCc1cccc2ccccc12</chem>          | Aromatic hydrocarbons |
| 2,5-dimethylphenol                   | <chem>Cc1ccc(C)c(O)c1</chem>           | Aromatic hydrocarbons |
| alpha-aminotoluene                   | <chem>NCc1ccccc1</chem>                | Aromatic hydrocarbons |
| pentylbenzene                        | <chem>CCCCCc1ccccc1</chem>             | Aromatic hydrocarbons |

Table 2: List of names, their SMILES notations, and families of the validation set that could be grouped into families

| Name                       | SMILES                                      | Family                |
|----------------------------|---------------------------------------------|-----------------------|
| phthalicaciddiethylester   | <chem>CCOC(=O)c1ccccc1C(=O)OCC</chem>       | Aromatic hydrocarbons |
| ethylbenzoate              | <chem>CCOC(=O)c1ccccc1</chem>               | Aromatic hydrocarbons |
| 2,6-dimethylpyridine       | <chem>Cc1cccc(C)n1</chem>                   | Aromatic hydrocarbons |
| phenylaceticacidethylester | <chem>CCOC(=O)Cc1ccccc1</chem>              | Aromatic hydrocarbons |
| 3-methylpyridine           | <chem>Cc1cccn1</chem>                       | Aromatic hydrocarbons |
| 2-methylpyridine           | <chem>Cc1cccn1</chem>                       | Aromatic hydrocarbons |
| 2-methylphenol             | <chem>Cc1ccccc1O</chem>                     | Aromatic hydrocarbons |
| 1,2,3-trimethylbenzene     | <chem>Cc1ccc(C)c1C</chem>                   | Aromatic hydrocarbons |
| o-methylaniline            | <chem>Cc1ccccc1N</chem>                     | Aromatic hydrocarbons |
| o-xylene                   | <chem>Cc1ccccc1C</chem>                     | Aromatic hydrocarbons |
| propylbenzene              | <chem>CCCc1ccccc1</chem>                    | Aromatic hydrocarbons |
| m-methylaniline            | <chem>Cc1ccc(N)c1</chem>                    | Aromatic hydrocarbons |
| n,n-diethylaniline         | <chem>CCN(CC)c1ccccc1</chem>                | Aromatic hydrocarbons |
| toluene                    | <chem>Cc1ccccc1</chem>                      | Aromatic hydrocarbons |
| 1-methylnaphthalene        | <chem>Cc1cccc2ccccc12</chem>                | Aromatic hydrocarbons |
| n-ethylaniline             | <chem>CCNc1ccccc1</chem>                    | Aromatic hydrocarbons |
| o-chlorotoluene            | <chem>Cc1ccccc1Cl</chem>                    | Aromatic hydrocarbons |
| sec-butylbenzene           | <chem>CCC(C)c1ccccc1</chem>                 | Aromatic hydrocarbons |
| m-xylene                   | <chem>Cc1ccc(C)c1</chem>                    | Aromatic hydrocarbons |
| butylbenzene               | <chem>CCCCc1ccccc1</chem>                   | Aromatic hydrocarbons |
| 4-methylphenol             | <chem>Cc1ccc(O)cc1</chem>                   | Aromatic hydrocarbons |
| o-dichlorobenzene          | <chem>Clc1ccccc1Cl</chem>                   | Aromatic hydrocarbons |
| chlorobenzene              | <chem>Clc1ccccc1</chem>                     | Aromatic hydrocarbons |
| 3,4-dimethylphenol         | <chem>Cc1ccc(O)cc1C</chem>                  | Aromatic hydrocarbons |
| 2,7-dimethylnaphthalene    | <chem>Cc1ccc2ccc(C)cc2c1</chem>             | Aromatic hydrocarbons |
| 2-methylnaphthalene        | <chem>Cc1ccc2ccccc2c1</chem>                | Aromatic hydrocarbons |
| phthalicaciddibutylester   | <chem>CCCCOC(=O)c1ccccc1C(=O)OCCCC</chem>   | Aromatic hydrocarbons |
| 4-methylpyridine           | <chem>Cc1ccncc1</chem>                      | Aromatic hydrocarbons |
| quinaldine                 | <chem>Cc1ccc2ccccc2n1</chem>                | Aromatic hydrocarbons |
| 1-chloronaphthalene        | <chem>Clc1ccc2ccccc12</chem>                | Aromatic hydrocarbons |
| 1,2,3-trichlorobenzene     | <chem>Clc1ccc(Cl)c1Cl</chem>                | Aromatic hydrocarbons |
| m-dichlorobenzene          | <chem>Clc1ccc(Cl)c1</chem>                  | Aromatic hydrocarbons |
| p-dichlorobenzene          | <chem>Clc1cc(Cl)cc1</chem>                  | Aromatic hydrocarbons |
| 1,2,4-trichlorobenzene     | <chem>Clc1cc(Cl)c(Cl)c1</chem>              | Aromatic hydrocarbons |
| 1,3,5-trichlorobenzene     | <chem>Clc1cc(Cl)cc(Cl)c1</chem>             | Aromatic hydrocarbons |
| benzylchloride             | <chem>ClCc1ccccc1</chem>                    | Aromatic hydrocarbons |
| 3-isopropyltoluene         | <chem>Cc1ccc(C(C)C)c1</chem>                | Aromatic hydrocarbons |
| 2,4-dimethylphenol         | <chem>Cc1ccc(O)c(C)c1</chem>                | Aromatic hydrocarbons |
| ethylbenzene               | <chem>CCc1ccccc1</chem>                     | Aromatic hydrocarbons |
| 3-methylphenol             | <chem>Cc1ccc(O)c1</chem>                    | Aromatic hydrocarbons |
| phenol                     | <chem>Oc1ccccc1</chem>                      | Aromatic hydrocarbons |
| isoquinoline               | <chem>c1ccc2cnccc2c1</chem>                 | Aromatic hydrocarbons |
| phenylacetylene            | <chem>C#Cc1ccccc1</chem>                    | Aromatic hydrocarbons |
| isobutylbenzene            | <chem>CC(C)Cc1ccccc1</chem>                 | Aromatic hydrocarbons |
| p-terphenyl                | <chem>c1ccc(-c2ccc(-c3ccccc3)cc2)cc1</chem> | Aromatic hydrocarbons |
| 1,3,5-triisopropylbenzene  | <chem>CC(C)c1cc(C(C)C)cc(C(C)C)c1</chem>    | Aromatic hydrocarbons |
| naphthalene                | <chem>c1ccc2ccccc2c1</chem>                 | Aromatic hydrocarbons |
| 1,3-diisopropylbenzene     | <chem>CC(C)c1ccc(C(C)C)c1</chem>            | Aromatic hydrocarbons |
| m-terphenyl                | <chem>c1ccc(-c2ccc(-c3ccccc3)c2)cc1</chem>  | Aromatic hydrocarbons |
| acridine                   | <chem>c1ccc2nc3ccccc3cc2c1</chem>           | Aromatic hydrocarbons |
| isopropylbenzene           | <chem>CC(C)c1ccccc1</chem>                  | Aromatic hydrocarbons |
| triphenylmethane           | <chem>c1ccc(C(c2ccccc2)c2ccccc2)cc1</chem>  | Aromatic hydrocarbons |
| phenylcyclohexane          | <chem>c1ccc(C2CCCCC2)cc1</chem>             | Aromatic hydrocarbons |

Table 2: List of names, their SMILES notations, and families of the validation set that could be grouped into families

| Name                                          | SMILES                                                | Family                |
|-----------------------------------------------|-------------------------------------------------------|-----------------------|
| 1-phenyl-2-propanol                           | <chem>CC(O)Cc1ccccc1</chem>                           | Aromatic hydrocarbons |
| diphenylmethane                               | <chem>c1ccc(Cc2ccccc2)cc1</chem>                      | Aromatic hydrocarbons |
| anthracene                                    | <chem>c1ccc2cc3ccccc3cc2c1</chem>                     | Aromatic hydrocarbons |
| phenanthrene                                  | <chem>c1ccc2c(c1)ccc1ccccc12</chem>                   | Aromatic hydrocarbons |
| 1,2,3,4-tetrahydronaphthalene                 | <chem>c1ccc2c(c1)CCCC2</chem>                         | Aromatic hydrocarbons |
| indane                                        | <chem>c1ccc2c(c1)CCC2</chem>                          | Aromatic hydrocarbons |
| bis(2-ethylhexyl)phthalate                    | <chem>CCCCC(CC)COC(=O)c1ccccc1C(=O)OCC(CC)CCCC</chem> | Aromatic hydrocarbons |
| biphenyl                                      | <chem>c1ccc(-c2ccccc2)cc1</chem>                      | Aromatic hydrocarbons |
| hexamethylbenzene                             | <chem>Cc1c(C)c(C)c(C)c(C)c1C</chem>                   | Aromatic hydrocarbons |
| n-methylaniline                               | <chem>CNc1ccccc1</chem>                               | Aromatic hydrocarbons |
| quinoline                                     | <chem>c1ccc2ncccc2c1</chem>                           | Aromatic hydrocarbons |
| 1,3,5-trimethylbenzene                        | <chem>Cc1cc(C)cc(C)c1</chem>                          | Aromatic hydrocarbons |
| indene                                        | <chem>C1=Cc2ccccc2C1</chem>                           | Aromatic hydrocarbons |
| pyridine                                      | <chem>c1ccncc1</chem>                                 | Aromatic hydrocarbons |
| tert-butylbenzene                             | <chem>CC(C)(C)c1ccccc1</chem>                         | Aromatic hydrocarbons |
| 2-phenyl-2-propanol                           | <chem>CC(C)(O)c1ccccc1</chem>                         | Aromatic hydrocarbons |
| p-cumylphenol                                 | <chem>CC(C)(c1ccccc1)c1ccc(O)cc1</chem>               | Aromatic hydrocarbons |
| phthalic acid dimethylester                   | <chem>COC(=O)c1ccccc1C(=O)OC</chem>                   | Aromatic hydrocarbons |
| 2-phenylethanol                               | <chem>OCCc1ccccc1</chem>                              | Aromatic hydrocarbons |
| n,n-dimethylaniline                           | <chem>CN(C)c1ccccc1</chem>                            | Aromatic hydrocarbons |
| 1,3-benzenedicarboxylic acid dimethylester    | <chem>COC(=O)c1cccc(C(=O)OC)c1</chem>                 | Aromatic hydrocarbons |
| dimethylterephthalate                         | <chem>COC(=O)c1ccc(C(=O)OC)cc1</chem>                 | Aromatic hydrocarbons |
| 1,2,4,5-tetramethylbenzene                    | <chem>Cc1cc(C)c(C)cc1C</chem>                         | Aromatic hydrocarbons |
| benzene                                       | <chem>c1ccccc1</chem>                                 | Aromatic hydrocarbons |
| benzoic acid methylester                      | <chem>COC(=O)c1ccccc1</chem>                          | Aromatic hydrocarbons |
| benzylalcohol                                 | <chem>OCc1ccccc1</chem>                               | Aromatic hydrocarbons |
| butylchloride                                 | <chem>CCCCl</chem>                                    | Chlorides             |
| tert-butylchloride                            | <chem>CC(C)(C)Cl</chem>                               | Chlorides             |
| 1,4-dichlorobutane                            | <chem>ClCCCCl</chem>                                  | Chlorides             |
| sec-butylchloride                             | <chem>CCC(C)Cl</chem>                                 | Chlorides             |
| 1-chloropentane                               | <chem>CCCCCl</chem>                                   | Chlorides             |
| 2,3-dichlorobutane                            | <chem>CC(Cl)C(C)Cl</chem>                             | Chlorides             |
| 1-chloro-2-methylpropane                      | <chem>CC(C)CCl</chem>                                 | Chlorides             |
| sec-butylcyclohexane                          | <chem>CCC(C)C1CCCCC1</chem>                           | Cyclic compounds      |
| n-propylcyclohexane                           | <chem>CCCC1CCCCC1</chem>                              | Cyclic compounds      |
| furan                                         | <chem>c1ccoc1</chem>                                  | Cyclic compounds      |
| methylcyclohexane                             | <chem>CC1CCCCC1</chem>                                | Cyclic compounds      |
| .alpha.-pinene                                | <chem>CC1=CCC2CC1C2(C)C</chem>                        | Cyclic compounds      |
| methylcyclopentane                            | <chem>CC1CCCC1</chem>                                 | Cyclic compounds      |
| dibenzo[b,d]furan                             | <chem>c1ccc2c(c1)oc1ccccc12</chem>                    | Cyclic compounds      |
| 2-methyl-1,3-dioxolane                        | <chem>CC1OCCO1</chem>                                 | Cyclic compounds      |
| 1,2-epoxybutane                               | <chem>CCC1CO1</chem>                                  | Cyclic compounds      |
| .beta.-pinene                                 | <chem>C=C1CCC2CC1C2(C)C</chem>                        | Cyclic compounds      |
| ethylcyclohexane                              | <chem>CCC1CCCCC1</chem>                               | Cyclic compounds      |
| .gamma.-terpinene                             | <chem>CC1=CCC(C(C)C)=CC1</chem>                       | Cyclic compounds      |
| bicyclohexyl                                  | <chem>C1CCC(C2CCCCC2)CC1</chem>                       | Cyclic compounds      |
| .alpha.-terpinene                             | <chem>CC1=CC=C(C(C)C)CC1</chem>                       | Cyclic compounds      |
| 2,2-dimethyl-3-methylenebicyclo[2.2.1]heptane | <chem>C=C1C2CCC(C2)C1(C)C</chem>                      | Cyclic compounds      |
| cyclopentane                                  | <chem>C1CCCC1</chem>                                  | Cyclic compounds      |

Table 2: List of names, their SMILES notations, and families of the validation set that could be grouped into families

| Name                                    | SMILES                                  | Family           |
|-----------------------------------------|-----------------------------------------|------------------|
| 2,5-dihydrofuran                        | <chem>C1=CCOC1</chem>                   | Cyclic compounds |
| 2-methylbenzofuran                      | <chem>Cc1cc2ccccc2o1</chem>             | Cyclic compounds |
| cyclohexane                             | <chem>C1CCCCC1</chem>                   | Cyclic compounds |
| cycloheptane                            | <chem>C1CCCCC1</chem>                   | Cyclic compounds |
| cyclooctane                             | <chem>C1CCCCCCC1</chem>                 | Cyclic compounds |
| isopropylcyclohexane                    | <chem>CC(C)C1CCCCC1</chem>              | Cyclic compounds |
| cyclohexene                             | <chem>C1=CCCCC1</chem>                  | Cyclic compounds |
| terpinolene                             | <chem>CC1=CCC(=C(C)C)CC1</chem>         | Cyclic compounds |
| cyclopentene                            | <chem>C1=CCCC1</chem>                   | Cyclic compounds |
| 2,5-dimethylfuran                       | <chem>Cc1ccc(C)o1</chem>                | Cyclic compounds |
| 2,2-dimethyloxirane                     | <chem>CC1(C)CO1</chem>                  | Cyclic compounds |
| 4-ethenylcyclohexene                    | <chem>C=CC1CC=CCC1</chem>               | Cyclic compounds |
| 1,1-dimethylcyclopentane                | <chem>CC1(C)CCCC1</chem>                | Cyclic compounds |
| tetrahydrofuran                         | <chem>C1CCOC1</chem>                    | Cyclic compounds |
| tetrahydropyran                         | <chem>C1CCOCC1</chem>                   | Cyclic compounds |
| n-butylcyclohexane                      | <chem>CCCCC1CCCCC1</chem>               | Cyclic compounds |
| 1,4-dioxane                             | <chem>C1COCCO1</chem>                   | Cyclic compounds |
| ethylacetoacetate                       | <chem>CCOC(=O)CC(C)=O</chem>            | Esters           |
| methylactate                            | <chem>COC(=O)C(C)O</chem>               | Esters           |
| methylacetoacetate                      | <chem>COC(=O)CC(C)=O</chem>             | Esters           |
| isopropenylacetate                      | <chem>C=C(C)OC(C)=O</chem>              | Esters           |
| salicylicacidmethylester                | <chem>COC(=O)c1ccccc1O</chem>           | Esters           |
| ethyleneglycolmonoethyletheracetate     | <chem>CCOCCOC(C)=O</chem>               | Esters           |
| diethylsuccinate                        | <chem>CCOC(=O)CCC(=O)OCC</chem>         | Esters           |
| 4-oxo-pentanoicacidethylester           | <chem>CCOC(=O)CCC(C)=O</chem>           | Esters           |
| alpha-hydroxy-isobutyricacidmethylester | <chem>COC(=O)C(C)(C)O</chem>            | Esters           |
| methacrylicacid,butylester              | <chem>C=C(C)C(=O)OCCCC</chem>           | Esters           |
| diethyleneglycolmonoethyletheracetate   | <chem>CCOCCOCCOC(C)=O</chem>            | Esters           |
| 2-methylpropanoicacidmethylester        | <chem>COC(=O)C(C)C</chem>               | Esters           |
| ethylacetate                            | <chem>CCOC(C)=O</chem>                  | Esters           |
| ethylmethacrylate                       | <chem>C=C(C)C(=O)OCC</chem>             | Esters           |
| dimethylglutarate                       | <chem>COC(=O)CCCC(=O)OC</chem>          | Esters           |
| dimethylsuccinate                       | <chem>COC(=O)CCC(=O)OC</chem>           | Esters           |
| diethylmalonate                         | <chem>CCOC(=O)CC(=O)OCC</chem>          | Esters           |
| methacrylicacidmethylester              | <chem>C=C(C)C(=O)OC</chem>              | Esters           |
| 1-methoxyisopropylacetate               | <chem>COCC(C)OC(C)=O</chem>             | Esters           |
| ethylactate                             | <chem>CCOC(=O)C(C)O</chem>              | Esters           |
| cyclohexylacetate                       | <chem>CC(=O)OC1CCCCC1</chem>            | Esters           |
| isobutylacetate                         | <chem>CC(=O)OCC(C)C</chem>              | Esters           |
| 1,2,3-propanetriol-triacetate           | <chem>CC(=O)OCC(COC(C)=O)OC(C)=O</chem> | Esters           |
| isoamylacetate                          | <chem>CC(=O)OCCC(C)C</chem>             | Esters           |
| ethyleneglycoldiacetate                 | <chem>CC(=O)OCCOC(C)=O</chem>           | Esters           |
| octadecanoicacidmethylester             | <chem>CCCCCCCCCCCCCCCCC(=O)OC</chem>    | Esters           |
| aceticacidphenylester                   | <chem>CC(=O)Oc1ccccc1</chem>            | Esters           |
| hexadecanoicacidethylester              | <chem>CCCCCCCCCCCCCCCCC(=O)OCC</chem>   | Esters           |
| hexadecanoicacidmethylester             | <chem>CCCCCCCCCCCCCCCCC(=O)OC</chem>    | Esters           |
| tetradecanoicacidethylester             | <chem>CCCCCCCCCCCCC(=O)OCC</chem>       | Esters           |
| tetradecanoicacidmethylester            | <chem>CCCCCCCCCCCCC(=O)OC</chem>        | Esters           |

Table 2: List of names, their SMILES notations, and families of the validation set that could be grouped into families

| Name                               | SMILES                                         | Family |
|------------------------------------|------------------------------------------------|--------|
| dodecanoicacidethylester           | <chem>CCCCCCCCCCCC(=O)OCC</chem>               | Esters |
| dodecanoicacidmethylester          | <chem>CCCCCCCCCCCC(=O)OC</chem>                | Esters |
| propanoicacidethylester            | <chem>CCOC(=O)CC</chem>                        | Esters |
| decanoicacidethylester             | <chem>CCCCCCCCC(=O)OCC</chem>                  | Esters |
| isobutylisobutyrate                | <chem>CC(C)COC(=O)C(C)C</chem>                 | Esters |
| isobutylformate                    | <chem>CC(C)COC=O</chem>                        | Esters |
| octanoicacidethylester             | <chem>CCCCCCCC(=O)OCC</chem>                   | Esters |
| octanoicacidmethylester            | <chem>CCCCCCCC(=O)OC</chem>                    | Esters |
| 2-ethylhexylacetate                | <chem>CCCCC(CC)COC(C)=O</chem>                 | Esters |
| tetrahydro-5-methyl-2-furano<br>ne | <chem>CC1CCC(=O)O1</chem>                      | Esters |
| methylpropanoate                   | <chem>CCC(=O)OC</chem>                         | Esters |
| propionicanhydride                 | <chem>CCC(=O)OC(=O)CC</chem>                   | Esters |
| isoamylbutyrate                    | <chem>CCCC(=O)OCCC(C)C</chem>                  | Esters |
| ethylbutyrate                      | <chem>CCCC(=O)OCC</chem>                       | Esters |
| butyricanhydride                   | <chem>CCCC(=O)OC(=O)CCC</chem>                 | Esters |
| methylbutanoate                    | <chem>CCCC(=O)OC</chem>                        | Esters |
| sec-butylacetate                   | <chem>CCC(C)OC(C)=O</chem>                     | Esters |
| decanoicacidmethylester            | <chem>CCCCCCCCC(=O)OC</chem>                   | Esters |
| aceticanhydride                    | <chem>CC(=O)OC(C)=O</chem>                     | Esters |
| aceticacidisopropylester           | <chem>CC(=O)OC(C)C</chem>                      | Esters |
| cyclohexylformate                  | <chem>O=COC1CCCCC1</chem>                      | Esters |
| ethylisobutyrate                   | <chem>CCOC(=O)C(C)C</chem>                     | Esters |
| diethyloxalate                     | <chem>CCOC(=O)C(=O)OCC</chem>                  | Esters |
| 2-propenoicacidmethylester         | <chem>C=CC(=O)OC</chem>                        | Esters |
| 2-propenoicacidethylester          | <chem>C=CC(=O)OCC</chem>                       | Esters |
| propylacrylate                     | <chem>C=CC(=O)OCCC</chem>                      | Esters |
| formicacidpropylester              | <chem>CCCOC=O</chem>                           | Esters |
| propylacetate                      | <chem>CCCOC(C)=O</chem>                        | Esters |
| butanoicacidpropylester            | <chem>CCCOC(=O)CCC</chem>                      | Esters |
| propanoicacidpropylester           | <chem>CCCOC(=O)CC</chem>                       | Esters |
| propylisobutyrate                  | <chem>CCCOC(=O)C(C)C</chem>                    | Esters |
| 2-propenoicacidbutylester          | <chem>C=CC(=O)OCCCC</chem>                     | Esters |
| 2-butoxyethylacetate               | <chem>CCCCOCCOC(C)=O</chem>                    | Esters |
| tert-butylacetate                  | <chem>CC(=O)OC(C)(C)C</chem>                   | Esters |
| butylacetate                       | <chem>CCCCOC(C)=O</chem>                       | Esters |
| formicacidbutylester               | <chem>CCCCOC=O</chem>                          | Esters |
| butanoicacidbutylester             | <chem>CCCCOC(=O)CCC</chem>                     | Esters |
| maleicanhydride                    | <chem>O=C1C=CC(=O)O1</chem>                    | Esters |
| octylacetate                       | <chem>CCCCCCCCOC(C)=O</chem>                   | Esters |
| heptylacetate                      | <chem>CCCCCCCOC(C)=O</chem>                    | Esters |
| vinylacetate                       | <chem>C=COC(C)=O</chem>                        | Esters |
| vinylpropionate                    | <chem>C=COC(=O)CC</chem>                       | Esters |
| decanedioicacid dibutylester       | <chem>CCCCOC(=O)CCCCCCCCC(=O)OC<br/>CCC</chem> | Esters |
| hexylacetate                       | <chem>CCCCCOC(C)=O</chem>                      | Esters |
| amylacetate                        | <chem>CCCCCOC(C)=O</chem>                      | Esters |
| amylformate                        | <chem>CCCCCOC=O</chem>                         | Esters |
| aceticacid2-propenylester          | <chem>C=CCOC(C)=O</chem>                       | Esters |
| 3-buten-2-olacetate                | <chem>C=CC(C)OC(C)=O</chem>                    | Esters |
| propanoicacidbutylester            | <chem>CCCCOC(=O)CC</chem>                      | Esters |
| amylbutyrate                       | <chem>CCCCCOC(=O)CCC</chem>                    | Esters |
| 1,2-dimethoxyethane                | <chem>COCCOC</chem>                            | Ethers |

Table 2: List of names, their SMILES notations, and families of the validation set that could be grouped into families

| Name                                   | SMILES                                                           | Family                |
|----------------------------------------|------------------------------------------------------------------|-----------------------|
| diphenylether                          | <chem>c1ccc(Oc2ccccc2)cc1</chem>                                 | Ethers                |
| methoxybenzene                         | <chem>COc1ccccc1</chem>                                          | Ethers                |
| triethyleneglycoldimethylether         | <chem>COCCOCCOCCOC</chem>                                        | Ethers                |
| diethyleneglycoldimethylether          | <chem>COCCOCCOC</chem>                                           | Ethers                |
| di-sec-butylether                      | <chem>CCC(C)OC(C)CC</chem>                                       | Ethers                |
| diethyleneglycoldiethylether           | <chem>CCOCCOCCOCC</chem>                                         | Ethers                |
| di-n-propylether                       | <chem>CCCOC</chem>                                               | Ethers                |
| ethoxybenzene                          | <chem>CCOc1ccccc1</chem>                                         | Ethers                |
| methylbutylether                       | <chem>CCCCOC</chem>                                              | Ethers                |
| diethoxymethane                        | <chem>CCOCOC</chem>                                              | Ethers                |
| ethylbutylether                        | <chem>CCCCOC</chem>                                              | Ethers                |
| ethyltert-butylether(etbe)             | <chem>CCOC(C)(C)C</chem>                                         | Ethers                |
| dibutylether                           | <chem>CCCCOCCCC</chem>                                           | Ethers                |
| 1,2-diethoxyethane                     | <chem>CCOCCOCC</chem>                                            | Ethers                |
| diethyleneglycoldibutylether           | <chem>CCCCOCCOCCOCCCC</chem>                                     | Ethers                |
| ethylpropylether                       | <chem>CCCOCC</chem>                                              | Ethers                |
| diethylether                           | <chem>CCOCC</chem>                                               | Ethers                |
| dipentylether                          | <chem>CCCCCOCCCCC</chem>                                         | Ethers                |
| methylpentylether                      | <chem>CCCCCOC</chem>                                             | Ethers                |
| di-tert-butylether                     | <chem>CC(C)(C)OC(C)(C)C</chem>                                   | Ethers                |
| diisobutylether                        | <chem>CC(C)COCC(C)C</chem>                                       | Ethers                |
| diisopropylether                       | <chem>CC(C)OC(C)C</chem>                                         | Ethers                |
| triethylorthoformate;triethoxymethane; | <chem>CCOC(OCC)OCC</chem>                                        | Ethers                |
| 1,1-diethoxyethane                     | <chem>CCOC(C)OCC</chem>                                          | Ethers                |
| methyltert-butylether(mtbe)            | <chem>COC(C)(C)C</chem>                                          | Ethers                |
| 2,5-dimethyltetrahydrofuran            | <chem>CC1CCC(C)O1</chem>                                         | Ethers                |
| ethyltert-amylether                    | <chem>CCOC(C)(C)CC</chem>                                        | Ethers                |
| 2,4,6-trimethyl-1,3,5-trioxane         | <chem>CC1OC(C)OC(C)O1</chem>                                     | Ethers                |
| 1,1-dimethoxyethane                    | <chem>COC(C)OC</chem>                                            | Ethers                |
| methyltert-amylether(tame)             | <chem>CCC(C)(C)OC</chem>                                         | Ethers                |
| butylvinylether                        | <chem>C=COCCCC</chem>                                            | Ethers                |
| perfluorononane                        | <chem>FC(F)(F)C(F)(F)C(F)(F)C(F)(F)C(F)(F)C(F)(F)C(F)(F)F</chem> | Fluorides             |
| perfluoro-n-octane                     | <chem>FC(F)(F)C(F)(F)C(F)(F)C(F)(F)C(F)(F)C(F)(F)C(F)(F)F</chem> | Fluorides             |
| 1,3-difluorobenzene                    | <chem>Fc1cccc(F)c1</chem>                                        | Fluorides             |
| perfluorohexane                        | <chem>FC(F)(F)C(F)(F)C(F)(F)C(F)(F)C(F)(F)C(F)(F)C(F)(F)F</chem> | Fluorides             |
| perfluoropentane                       | <chem>FC(F)(F)C(F)(F)C(F)(F)C(F)(F)C(F)(F)C(F)(F)F</chem>        | Fluorides             |
| perfluorobutane                        | <chem>FC(F)(F)C(F)(F)C(F)(F)C(F)(F)C(F)(F)F</chem>               | Fluorides             |
| perfluorocyclobutane[rc318]            | <chem>FC1(F)C(F)(F)C(F)(F)C1(F)F</chem>                          | Fluorides             |
| 1,4-difluorobenzene                    | <chem>Fc1ccc(F)cc1</chem>                                        | Fluorides             |
| fluorobenzene                          | <chem>Fc1ccccc1</chem>                                           | Fluorides             |
| 1,2-difluorobenzene                    | <chem>Fc1ccccc1F</chem>                                          | Fluorides             |
| 1,1,1,3,3-pentafluorobutane            | <chem>CC(F)(F)CC(F)(F)F</chem>                                   | Fluorides             |
| perfluoro-n-heptane                    | <chem>FC(F)(F)C(F)(F)C(F)(F)C(F)(F)C(F)(F)C(F)(F)C(F)(F)F</chem> | Fluorides             |
| hexafluorobenzene                      | <chem>Fc1c(F)c(F)c(F)c(F)c1F</chem>                              | Fluorides             |
| iodobenzene                            | <chem>Ic1ccccc1</chem>                                           | Halogenated compounds |

Table 2: List of names, their SMILES notations, and families of the validation set that could be grouped into families

| Name                                 | SMILES                                     | Family                   |
|--------------------------------------|--------------------------------------------|--------------------------|
| 1-iodobutane                         | <chem>CCCCI</chem>                         | Halogenated compounds    |
| bromobenzene                         | <chem>BrC1ccccc1</chem>                    | Halogenated compounds    |
| butylbromide                         | <chem>CCCCBr</chem>                        | Halogenated compounds    |
| p-dibromobenzene                     | <chem>BrC1cc(Br)cc1</chem>                 | Halogenated compounds    |
| benzophenone                         | <chem>O=C(c1ccccc1)c1ccccc1</chem>         | Ketones                  |
| 2-cyclohexen-1-one                   | <chem>O=C1C=CCCC1</chem>                   | Ketones                  |
| methylisopropylketone                | <chem>CC(=O)C(C)C</chem>                   | Ketones                  |
| 3,3-dimethyl-2-butanone              | <chem>CC(=O)C(C)(C)C</chem>                | Ketones                  |
| 4-methyl-3-penten-2-one              | <chem>CC(=O)C=C(C)C</chem>                 | Ketones                  |
| 4-methyl-2-pentanone                 | <chem>CC(=O)CC(C)C</chem>                  | Ketones                  |
| acetophenone                         | <chem>CC(=O)c1ccccc1</chem>                | Ketones                  |
| 2,4-dimethyl-3-pentanone             | <chem>CC(C)C(=O)C(C)C</chem>               | Ketones                  |
| cyclohexanone                        | <chem>O=C1CCCCC1</chem>                    | Ketones                  |
| 2-nonanone                           | <chem>CCCCCCCC(C)=O</chem>                 | Ketones                  |
| 2-octanone                           | <chem>CCCCCCC(C)=O</chem>                  | Ketones                  |
| 2-heptanone                          | <chem>CCCCC(C)=O</chem>                    | Ketones                  |
| 3,5,5-trimethyl-2-cyclohexen-1-one   | <chem>CC1=CC(=O)CC(C)(C)C1</chem>          | Ketones                  |
| 2-hexanone                           | <chem>CCCCC(C)=O</chem>                    | Ketones                  |
| diisobutylketone                     | <chem>CC(C)CC(=O)CC(C)C</chem>             | Ketones                  |
| 5-nonanone                           | <chem>CCCCC(=O)CCCC</chem>                 | Ketones                  |
| 2-butanone                           | <chem>CCC(C)=O</chem>                      | Ketones                  |
| 4-heptanone                          | <chem>CCCC(=O)CCC</chem>                   | Ketones                  |
| 3-heptanone                          | <chem>CCCCC(=O)CC</chem>                   | Ketones                  |
| 2-pentanone                          | <chem>CCCC(C)=O</chem>                     | Ketones                  |
| methylvinylketone                    | <chem>C=CC(C)=O</chem>                     | Ketones                  |
| 3-hexanone                           | <chem>CCCC(=O)CC</chem>                    | Ketones                  |
| 3-methoxypropionitrile               | <chem>COCCC#N</chem>                       | Nitriles                 |
| allylcyanide                         | <chem>C=CCC#N</chem>                       | Nitriles                 |
| benzonitrile                         | <chem>N#Cc1ccccc1</chem>                   | Nitriles                 |
| benzylcyanide                        | <chem>N#CCc1ccccc1</chem>                  | Nitriles                 |
| glutaronitrile                       | <chem>N#CCCCC#N</chem>                     | Nitriles                 |
| hexanenitrile                        | <chem>CCCCC#N</chem>                       | Nitriles                 |
| isobutyronitrile                     | <chem>CC(C)C#N</chem>                      | Nitriles                 |
| diphenylcarbonate                    | <chem>O=C(Oc1ccccc1)Oc1ccccc1</chem>       | Other compounds          |
| nitrobenzene                         | <chem>O=[N+]([O-])c1ccccc1</chem>          | Other compounds          |
| m-nitrotoluene                       | <chem>Cc1cccc([N+]([O-])=O)c1</chem>       | Other compounds          |
| di-tert.butylperoxide                | <chem>CC(C)(C)OOC(C)(C)C</chem>            | Other compounds          |
| hexamethylphosphoricacidtri<br>amide | <chem>CN(C)P(=O)(N(C)C)N(C)C</chem>        | Other compounds          |
| tert.butylhydroperoxide              | <chem>CC(C)(C)OO</chem>                    | Other compounds          |
| triethylphosphate                    | <chem>CCOP(=O)(OCC)OCC</chem>              | Other compounds          |
| 2,4-toluenediisocyanate              | <chem>Cc1ccc(N=C=O)cc1N=C=O</chem>         | Other compounds          |
| carbonicaciddiethylester             | <chem>CCOC(=O)OCC</chem>                   | Other compounds          |
| isocyanicacidbutylester              | <chem>CCCCN=C=O</chem>                     | Other compounds          |
| triethoxyphosphine                   | <chem>CCOP(OCC)OCC</chem>                  | Other compounds          |
| hexamethylenediisocyanate            | <chem>O=C=NCCCCCN=C=O</chem>               | Other compounds          |
| o-nitrotoluene                       | <chem>Cc1ccccc1[N+](=O)[O-]</chem>         | Other compounds          |
| diethyleneglycolmonomethyle<br>ther  | <chem>COCCOCCO</chem>                      | Polyfunctional compounds |
| 2-methoxyphenol                      | <chem>COc1ccccc1O</chem>                   | Polyfunctional compounds |
| triphenylphosphine                   | <chem>c1ccc(P(c2ccccc2)c2ccccc2)cc1</chem> | Polyfunctional compounds |
| 3,4-dichlorophenylisocyanate         | <chem>O=C=Nc1ccc(Cl)c(Cl)c1</chem>         | Polyfunctional compounds |

Table 2: List of names, their SMILES notations, and families of the validation set that could be grouped into families

| Name                                | SMILES                                          | Family                   |
|-------------------------------------|-------------------------------------------------|--------------------------|
| 1-tert-butoxy-2-propanol            | <chem>CC(O)COC(C)(C)C</chem>                    | Polyfunctional compounds |
| 2-methoxy-1-propanol                | <chem>COC(C)CO</chem>                           | Polyfunctional compounds |
| 5-hydroxymethylfurfural             | <chem>O=Cc1ccc(CO)o1</chem>                     | Polyfunctional compounds |
| salicylaldehyde                     | <chem>O=Cc1ccccc1O</chem>                       | Polyfunctional compounds |
| furfural                            | <chem>O=Cc1ccco1</chem>                         | Polyfunctional compounds |
| sulfolane                           | <chem>O=S1(=O)CCCC1</chem>                      | Polyfunctional compounds |
| 3,4-dichloronitrobenzene            | <chem>O=[N+](=[O-])c1ccc(Cl)c(Cl)c1</chem>      | Polyfunctional compounds |
| p-chlorophenol                      | <chem>Oc1ccc(Cl)cc1</chem>                      | Polyfunctional compounds |
| tetrahydrofurfuryl alcohol          | <chem>OCC1CCCO1</chem>                          | Polyfunctional compounds |
| diacetonealcohol                    | <chem>CC(=O)CC(C)(C)O</chem>                    | Polyfunctional compounds |
| p-methoxyphenol                     | <chem>COc1ccc(O)cc1</chem>                      | Polyfunctional compounds |
| levulinic acid                      | <chem>CC(=O)CCC(=O)O</chem>                     | Polyfunctional compounds |
| methylethylketoxime                 | <chem>CCC(C)=NO</chem>                          | Polyfunctional compounds |
| 8-hydroxyquinoline                  | <chem>Oc1cccc2ccncc12</chem>                    | Polyfunctional compounds |
| o-chlorophenol                      | <chem>Oc1ccccc1Cl</chem>                        | Polyfunctional compounds |
| furfuryl alcohol                    | <chem>OCc1ccco1</chem>                          | Polyfunctional compounds |
| cyanoacetic acid ethylester         | <chem>CCOC(=O)CC#N</chem>                       | Polyfunctional compounds |
| 1-methoxy-2-propanol                | <chem>COCC(C)O</chem>                           | Polyfunctional compounds |
| p-phenetidine                       | <chem>CCOc1ccc(N)cc1</chem>                     | Polyfunctional compounds |
| 1-propoxy-2-propanol                | <chem>CCCOCC(C)O</chem>                         | Polyfunctional compounds |
| ethyleneglycolmonopropylether       | <chem>CCCOCCO</chem>                            | Polyfunctional compounds |
| bis(2-chloroethyl) ether            | <chem>ClCCOCCCl</chem>                          | Polyfunctional compounds |
| 1,2-propyleneglycol1-monobutylether | <chem>CCCCOCC(C)O</chem>                        | Polyfunctional compounds |
| diethyleneglycolmonopropylether     | <chem>CCCOCCOCCO</chem>                         | Polyfunctional compounds |
| n-methyl-2-pyrrolidone              | <chem>CN1CCCC1=O</chem>                         | Polyfunctional compounds |
| 1,3-dimethylimidazolidin-2-one      | <chem>CN1CCN(C)C1=O</chem>                      | Polyfunctional compounds |
| chloroacetic acid ethylester        | <chem>CCOC(=O)CCl</chem>                        | Polyfunctional compounds |
| morpholine                          | <chem>C1COCCN1</chem>                           | Polyfunctional compounds |
| dipropyleneglycolbutylether         | <chem>CCCCOCC(C)OCC(C)O</chem>                  | Polyfunctional compounds |
| 2-butoxyethanol                     | <chem>CCCCOCCO</chem>                           | Polyfunctional compounds |
| n-ethyl-2-pyrrolidone               | <chem>CCN1CCCC1=O</chem>                        | Polyfunctional compounds |
| diethyleneglycolmonobutylether      | <chem>CCCCOCCOCCO</chem>                        | Polyfunctional compounds |
| 4-ethylmorpholine                   | <chem>CCN1CCOCC1</chem>                         | Polyfunctional compounds |
| eugenol                             | <chem>C=CCc1ccc(O)c(OC)c1</chem>                | Polyfunctional compounds |
| p-chloroaniline                     | <chem>Nc1ccc(Cl)cc1</chem>                      | Polyfunctional compounds |
| diethyleneglycoln-hexylether        | <chem>CCCCCOCCOCCO</chem>                       | Polyfunctional compounds |
| benzoylchloride                     | <chem>O=C(Cl)c1ccccc1</chem>                    | Polyfunctional compounds |
| 2-ethoxyethanol                     | <chem>CCOCCO</chem>                             | Polyfunctional compounds |
| diethyleneglycolethylether          | <chem>CCOCCOCCO</chem>                          | Polyfunctional compounds |
| 1-ethoxy-2-propanol                 | <chem>CCOCC(C)O</chem>                          | Polyfunctional compounds |
| trichlorophenylsilane               | <chem>Cl[Si](Cl)(Cl)c1ccccc1</chem>             | Silanes/siloxanes        |
| tetramethylsilane                   | <chem>C[Si](C)(C)C</chem>                       | Silanes/siloxanes        |
| hexamethyldisilazane                | <chem>C[Si](C)(C)N[Si](C)(C)C</chem>            | Silanes/siloxanes        |
| tetramethoxysilane                  | <chem>CO[Si](OC)(OC)OC</chem>                   | Silanes/siloxanes        |
| tetraethylsilane                    | <chem>CC[Si](CC)(CC)CC</chem>                   | Silanes/siloxanes        |
| hexamethyldisiloxane                | <chem>C[Si](C)(C)O[Si](C)(C)C</chem>            | Silanes/siloxanes        |
| dichlorodiethylsilane               | <chem>CC[Si](Cl)(Cl)CC</chem>                   | Silanes/siloxanes        |
| octamethyltrisiloxane               | <chem>C[Si](C)(C)O[Si](C)(C)O[Si](C)(C)C</chem> | Silanes/siloxanes        |

Table 2: List of names, their SMILES notations, and families of the validation set that could be grouped into families

| Name                         | SMILES                                                                           | Family              |
|------------------------------|----------------------------------------------------------------------------------|---------------------|
| octamethylcyclotetrasiloxane | <chem>C[Si]1(C)O[Si](C)(C)O[Si](C)(C)O[Si](C)(C)O1</chem>                        | Silanes/siloxanes   |
| dichloromethylphenylsilane   | <chem>C[Si](Cl)(Cl)c1ccccc1</chem>                                               | Silanes/siloxanes   |
| dodecamethylpentasiloxane    | <chem>C[Si](C)(C)O[Si](C)(C)O[Si](C)(C)O[Si](C)(C)O[Si](C)(C)O[Si](C)(C)C</chem> | Silanes/siloxanes   |
| decamethyltetrasiloxane      | <chem>C[Si](C)(C)O[Si](C)(C)O[Si](C)(C)O[Si](C)(C)O[Si](C)(C)C</chem>            | Silanes/siloxanes   |
| tetraethoxysilane            | <chem>CCO[Si](OCC)(OCC)OCC</chem>                                                | Silanes/siloxanes   |
| benzo(b)thiophene            | <chem>c1ccc2sccc2c1</chem>                                                       | Sulfides/thiophenes |
| dipropylsulfide              | <chem>CCCSCCC</chem>                                                             | Sulfides/thiophenes |
| 2-methylthiophene            | <chem>Cc1cccs1</chem>                                                            | Sulfides/thiophenes |
| thiophene                    | <chem>c1ccsc1</chem>                                                             | Sulfides/thiophenes |
| 2,5-dimethylthiophene        | <chem>Cc1ccc(C)s1</chem>                                                         | Sulfides/thiophenes |
| diethylsulfide               | <chem>CCSCC</chem>                                                               | Sulfides/thiophenes |
| diethyldisulfide             | <chem>CCSSCC</chem>                                                              | Sulfides/thiophenes |
| 2-ethylthiophene             | <chem>CCc1cccs1</chem>                                                           | Sulfides/thiophenes |
| tetrahydrothiophene          | <chem>C1CCSC1</chem>                                                             | Sulfides/thiophenes |
| allylsulfide                 | <chem>C=CCSCC=C</chem>                                                           | Sulfides/thiophenes |
| 3-methylthiophene            | <chem>Cc1ccsc1</chem>                                                            | Sulfides/thiophenes |
| n-butylmercaptan             | <chem>CCCCS</chem>                                                               | Thiols              |
| benzenethiol                 | <chem>Sc1ccccc1</chem>                                                           | Thiols              |
| 2-methyl-2-propanethiol      | <chem>CC(C)(C)S</chem>                                                           | Thiols              |
| 1-pentanethiol               | <chem>CCCCCS</chem>                                                              | Thiols              |
| iso-butylmercaptan           | <chem>CC(C)CS</chem>                                                             | Thiols              |
